# Supplementary material for: S$^2$Contact: Graph-based Network for 3D Hand-Object Contact Estimation with Semi-Supervised Learning
Source: arXiv:2208.00874 source file (2023-08-03)
Supplement: Supplementary file 1 [file supplementary.tex]

In this supplemental document, we present:
\begin{enumerate}
    \item implementation details of GCN-Contact (Section \ref{sec:implementation});
    \item ablations on pseudo-labels (Section \ref{sec:pseudo-labels});
    \item comparison with state-of-the-arts (Section \ref{sec:SOTA});
    \item additional qualitative examples (Section \ref{sec:qualitative});
    \item complete performances of different GCN-Contact design choices (Section \ref{sec:ablation_graph});
    \item complete table for computational analysis (Section \ref{sec:computational}).
\end{enumerate}

Note that all the notation and abbreviations here are consistent with the main manuscript. 

\section{Implementation details of GCN-Contact} \label{sec:implementation}
The network architecture is illustrated in Table \ref{table:network_architecture}.

\begin{figure}[h]
\centering
% \vspace{+0.1cm}
\includegraphics[width=1\linewidth]{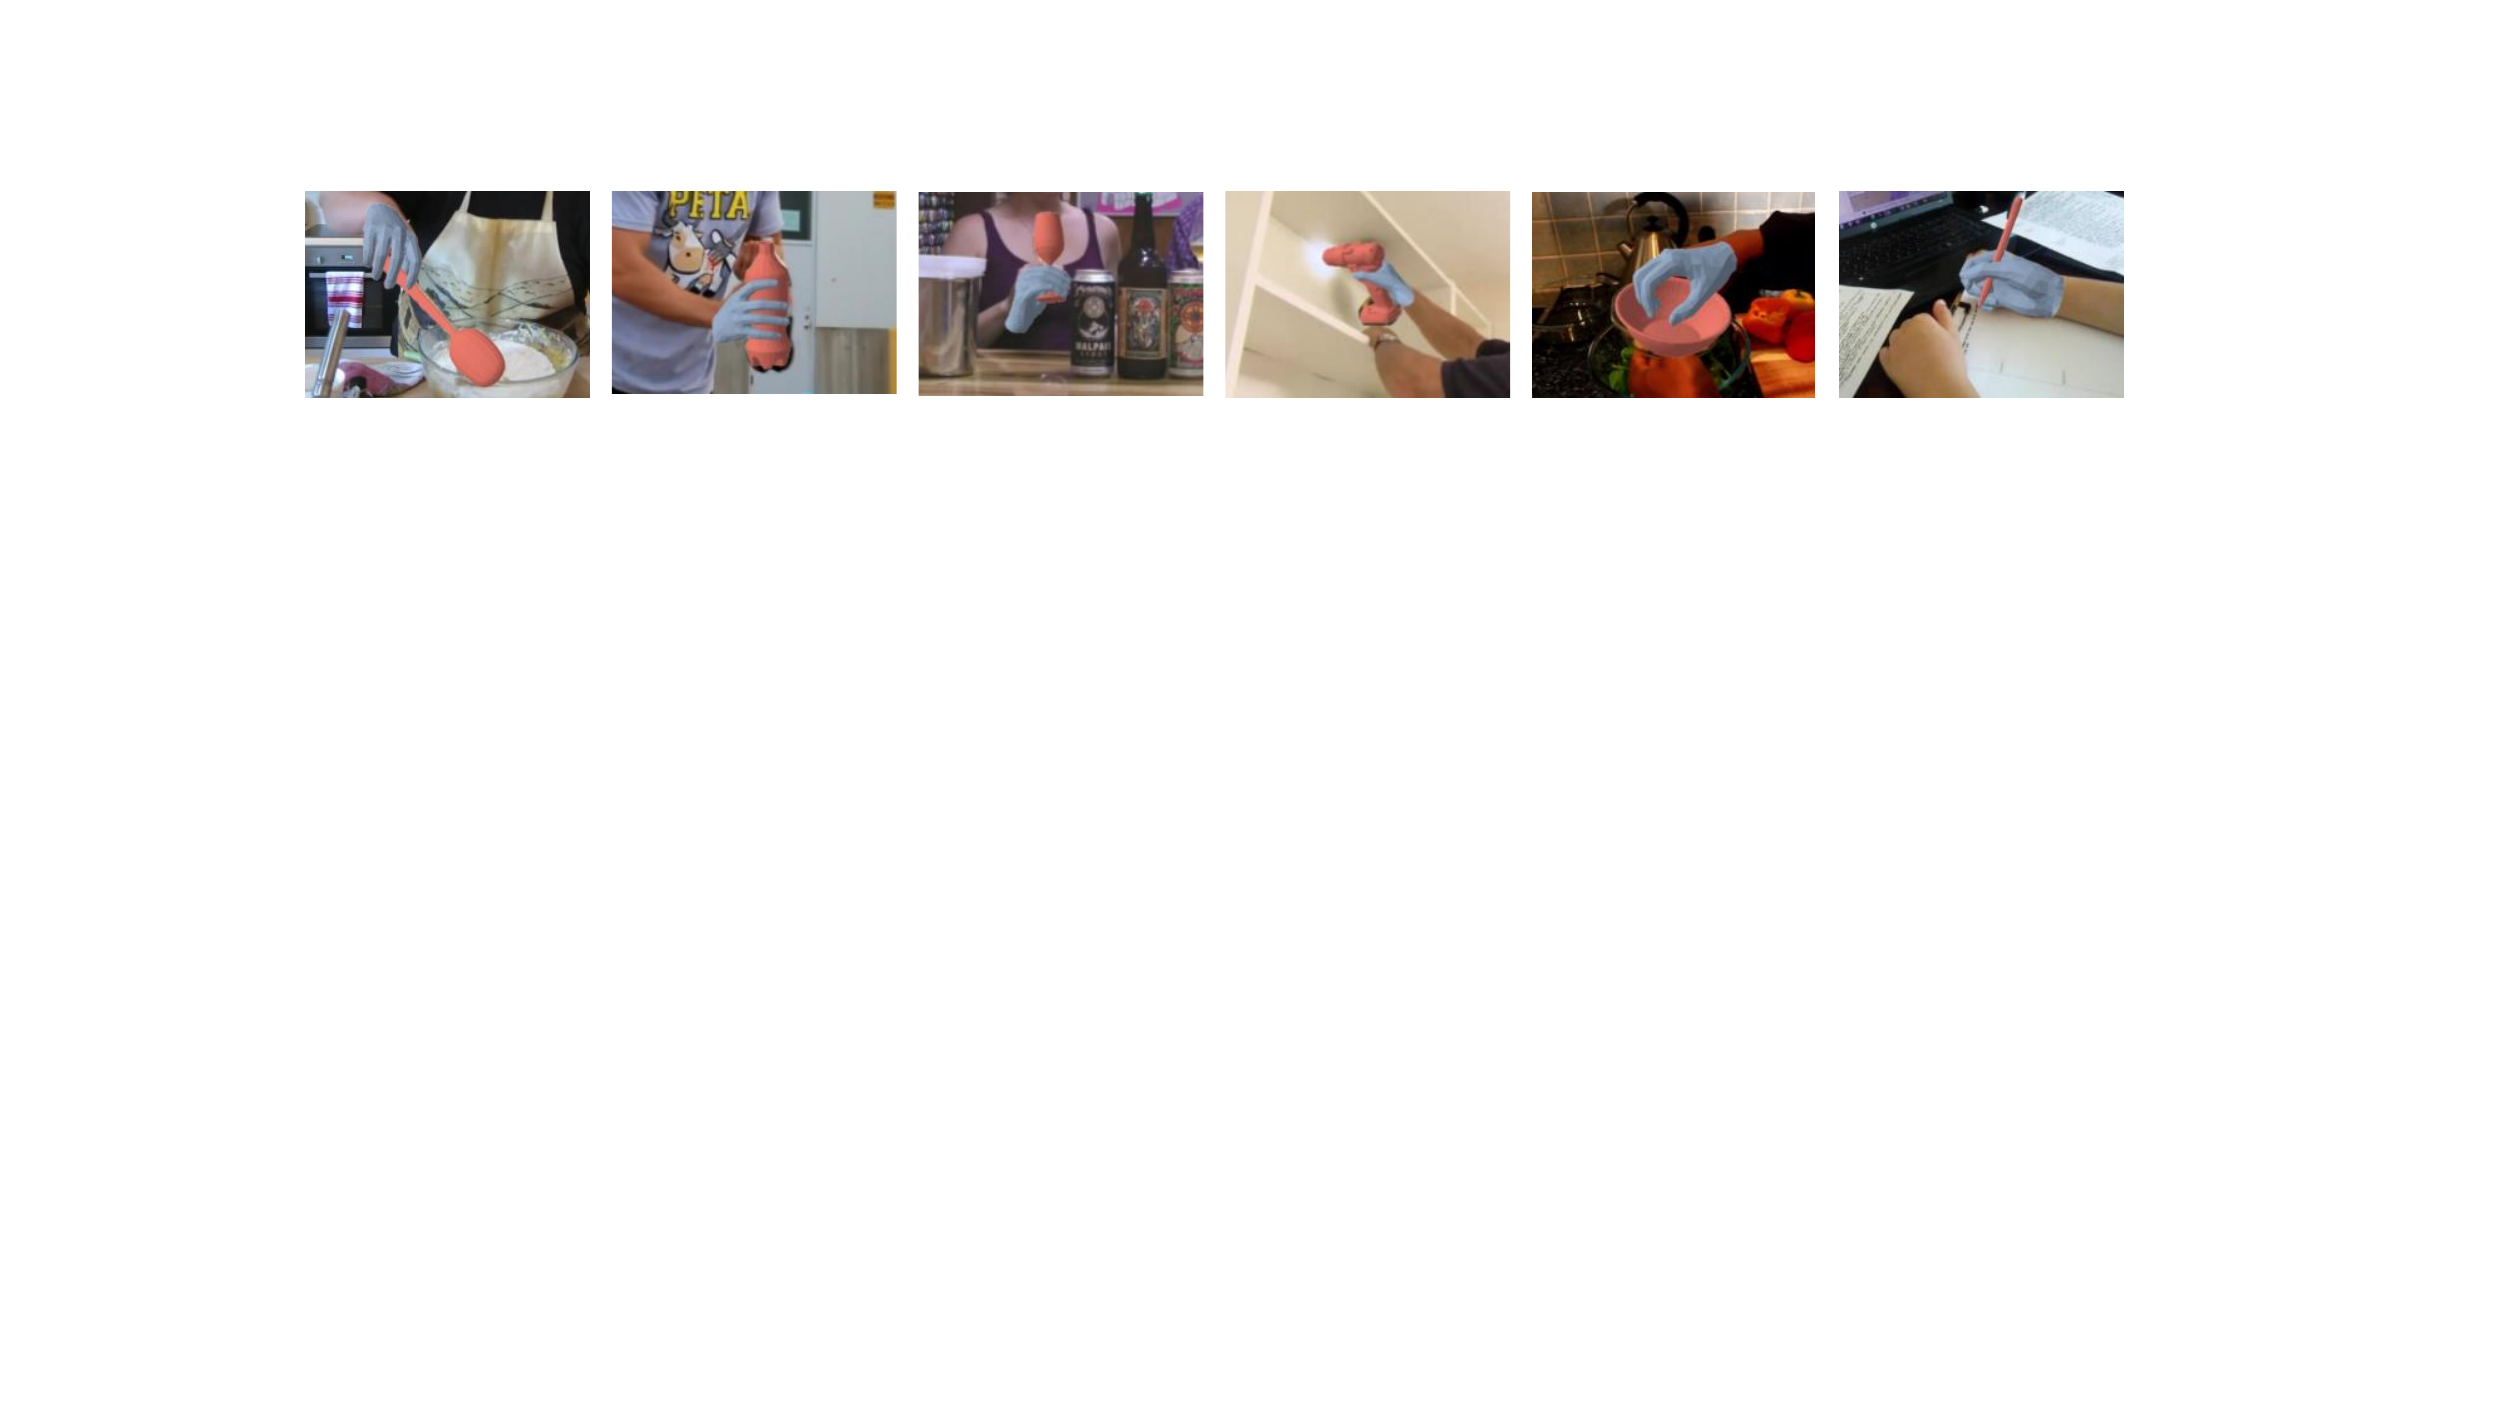}
% \vspace{-0.7cm}
\caption{
Qualitative results on \emph{EPIC-Kitchens}~\cite{Damen2018EPICKITCHENS} and \emph{100 Days of Hands}~\cite{Shan20}.
}
% \vspace{-0.4cm}
\label{fig:vis_in_the_wild}
\end{figure}

\section{Ablations on pseudo-labels} \label{sec:pseudo-labels}

\subsection{Effects of varying thresholds for pseudo-labels generation}
We study the effect of different thresholds of the pseudo-labels filtering mechanism on \emph{HO-3D} in Figure~\ref{fig:threthold1} and Figure~\ref{fig:threshold2}. As shown in Figure~\ref{fig:threthold1}, the performance
is higher than the method without Chamfer distance by large margins when $60<t_{dist}\leq80$. Note that the performance peaks at $t_{dist}=70$. When $t_{dist}>70$, further
increasing $t_{dist}$ led to a drastic drop in pseudo-label as hand and object are so far away from each other such that the resulting pseudo-labels are in low-quality. 
On the contrary, when $t_{dist}\leq60$, there are less qualifying pseudo-labels leading to performance drop from insufficient training labels.
% the performance 
% drops due to tougher requirements leading to insufficient pseudo-labels for training.
% to select a sufficient number of pseudo-labels. 
% Similar situation for $t_{pen}$ and $t_{SSIM}$.
We obtain similar observations for $t_{pen}$ and $t_{SSIM}$.

\subsection{Amounts of pseudo-labels}

We analyse the effect of using different fractions of pseudo-labels in semi-supervised learning on \emph{HO-3D} in Figure~\ref{fig:amounts}. We uniformly sample 20\%, 40\%, 60\%, and 80\% of the collected pseudo-labels for semi-supervised learning. As shown, the performance has been significantly improved after adding 20\% of pseudo-labels. We observe that the more pseudo-labels used in training, the better the performance the model can achieve.

% \subsection{Statistics of pseudo-labels}
% \zq{It seems similar with 2.1}

\section{Comparison with state-of-the-arts} \label{sec:SOTA}
We compare against the state-of-the-art approaches [3,17,18] on \emph{HO-3D} in Table \ref{table:semisupervised}. [3] is an optimisation-based method which leverages 2D image cues and 3D contact priors for reconstructing hand-object interactions. [17] uses a feed-forward neural network to predict 3D hand pose and object pose where its single-frame model with full 3D supervision. 
% (\zq{[17] has been reported in submission paper, in Table2 it's the initial pose}) 
[18] follows a fitting-based approach which builds on estimates from neural network models for detection, object segmentation and 3D hand pose estimation trained with full supervision.

\section{Additional qualitative examples} \label{sec:qualitative}
In this section, we show additional qualitative results. In Figure \ref{fig:sup_vis_contactpose}, we visualise the predictions of ContactOpt~[13] and our method as well as the ground-truth. We can see that our method is able to better reconstruction hand and object with more accurate contact map estimations. Our method performs significantly
better than previous approaches. In Figure~\ref{fig:sup_vis_ho3d}, we show more examples of our method and [30] on \emph{HO-3D}. Our method significantly improve the hand-object pose. The last row of Figure~\ref{fig:sup_vis_ho3d} shows a failure case where the region of hand-object contact was too small for the network to produce a good contact prediction.

We provide qualitative examples on out-of-domain objects in Figure~\ref{fig:vis_in_the_wild}.

\section{Performances of different GCN-Contact design choices} \label{sec:ablation_graph}
Complete results are reported in Table \ref{table:ab_graph}.

\section{Computational analysis} \label{sec:computational}
Complete results are reported in Table \ref{table:runtime}.
% Please add the following required packages to your document preamble:
\newcolumntype{C}{>{\centering\arraybackslash}X}
\begin{table}[h]
\begin{center}
% \vspace{-0.2cm}
\caption{Comparison on computational requirements of different networks.}
\label{table:runtime}
% \vspace{-0.2cm}
\resizebox{0.9\linewidth}{!}{%
\begin{tabularx}{\linewidth}{l | C | C | C }
\toprule
 & Baseline & DGCNN \cite{wang2019dynamic} & Ours \\ 
\midrule 
Parameters & {\footnotesize1,424,138} &{\footnotesize530,442} & {\footnotesize587,658} \\
GPU memory (GB) & {\footnotesize13.3} & {\footnotesize21.1} & {\footnotesize10.4} \\
\bottomrule
\end{tabularx}
}
% \vspace{-0.6cm}
\end{center}
\end{table}
